# Supplementary material for: Quality Assured: Rethinking Annotation Strategies in Imaging AI
Source: arXiv:2407.17596 source file (2024-07-26)
Supplement: Supplementary file 1 [file instruction_01_minimal_text.pdf]

# Overview

- Terminology ..... 2
- Goal..... 3
- Occlusion..... 4
- Medical instruments..... 5
- Medical instruments - Holes..... 6
- Medical instruments - Transparency..... 7

# Terminology

## **Definition “Matter”:**

- Anything that has mass, takes up space and can be clearly identified.
- Examples: tissue, surgical tools, blood

# Goal - Detect and segment all relevant medical instruments

## **Only segment medical instruments**

- Each medical instrument is their own instance.
- Each instance has their own colour.
- The interior of a segmentation represents a medical instrument.
- Everything outside the medical instrument segmentations is regarded as other matter.

# Occlusion

Each pixel may correspond to exactly one instance.

The solid/liquid matter that occurs first along the line of sight of the endoscope determines the label.

# Medical instruments

## **Definition “Medical instrument”:**

- An elongated rigid object placed inside the patient and manipulated from outside the patient.
- Examples: grasper, scalpel, (transparent) trocar, clip applicator, hooks, stapling device, suction

# Medical instruments - Holes

Several medical instruments feature holes.  
They are regarded as part of the instrument.

# Medical instruments - Transparency

Medical instruments may be transparent.

The occlusion rule holds in this case as well.
