# Supplementary material for: Quality Assured: Rethinking Annotation Strategies in Imaging AI
Source: arXiv:2407.17596 source file (2024-07-26)
Supplement: Supplementary file 2 [file instruction_02_extended_text.pdf]

# Overview

|                                              |    |
|----------------------------------------------|----|
| • Terminology.....                           | 2  |
| • Goal.....                                  | 3  |
| • Occlusion.....                             | 4  |
| • Medical instruments.....                   | 5  |
| • Medical instruments - Holes.....           | 6  |
| • Medical instruments - Holes exception..... | 7  |
| • Medical instruments - Transparency.....    | 8  |
| • Text overlay.....                          | 9  |
| • Image overlay.....                         | 10 |

# Terminology

## **Definition “Matter”:**

- Anything that has mass, takes up space and can be clearly identified.
- Examples: tissue, surgical tools, blood
- Counterexamples: reflections, digital overlays, movement artifacts, smoke

# Goal - Detect and segment all relevant medical instruments

## **Only segment medical instruments**

- Each medical instrument is their own instance.
- If two parts of the same instrument are visible, they belong to the same instrument instance.
- Each instance has their own colour.
- The interior of a segmentation represents a medical instrument.
- Everything outside the medical instrument segmentations is regarded as other matter.
- Be as precise as possible. Every pixel counts in surgery.

# Occlusion

Each pixel may correspond to exactly one instance.

The solid/liquid matter that occurs first along the line of sight of the endoscope determines the label.

This may result in multiple segmentations for a single instrument that is occluded by another instrument, blood or tissue, for example.

# Medical instruments

## **Definition “Medical instrument”:**

- An elongated rigid object placed inside the patient and manipulated from outside the patient.
- Examples: grasper, scalpel, (transparent) trocar, clip applicator, hooks, stapling device, suction
- Counterexamples: non-rigid tubes, bandage, compress, needle (not directly manipulated from outside but manipulated with an instrument), coagulation sponges, metal clips

# Medical instruments - Holes

Several medical instruments feature holes.  
They are regarded as part of the instrument.

A hole is made up of pixels that do not show  
parts of the instrument but are either

- type a) completely surrounded by pixels of the same instrument or

- type b) completely surrounded by pixels of one instrument and the margin of the instrument would close the hole outside the image.

# Medical instruments - Holes exception

The sole exception are trocars when the camera is placed inside them.

Trocars are transparent medical instruments

- They are placed through the abdomen.
- They function as a portal for the other medical instruments.
- When the camera is inside a trocar, a trocar can take up a large part of the image.

Trocars are exempt from the hole rule

- Reason: Otherwise, the holes would make up a large part of the image.

# Medical instruments - Transparency

Medical instruments may be transparent.  
The occlusion rule holds in this case as well.



# Text overlay

Text overlay is text that is visible in the image.  
The background of the text is the regular image.

Text overlay shall be ignored.

# Image overlay

Image overlay is often uniform coloured shapes that overlay with the image.

Text with an added uniform color background is considered as image overlay.

Image overlay is treated like “other matter” and should not be part of the segmentation.
