# Supplementary material for: Quality Assured: Rethinking Annotation Strategies in Imaging AI
Source: arXiv:2407.17596 source file (2024-07-26)
Supplement: Supplementary file 3 [file instruction_03_picture_version.pdf]

# Overview

|                                              |    |
|----------------------------------------------|----|
| • Terminology.....                           | 2  |
| • Goal.....                                  | 3  |
| • Occlusion.....                             | 5  |
| • Medical instruments.....                   | 6  |
| • Medical instruments - Holes.....           | 11 |
| • Medical instruments - Holes exception..... | 12 |
| • Medical instruments - Transparency.....    | 14 |
| • Text overlay.....                          | 15 |
| • Image overlay.....                         | 16 |

# Terminology

## Definition “Matter”:

- Anything that has mass, takes up space and can be clearly identified.
- Examples: tissue, surgical tools, blood
- Counterexamples: reflections, digital overlays, movement artifacts, smoke

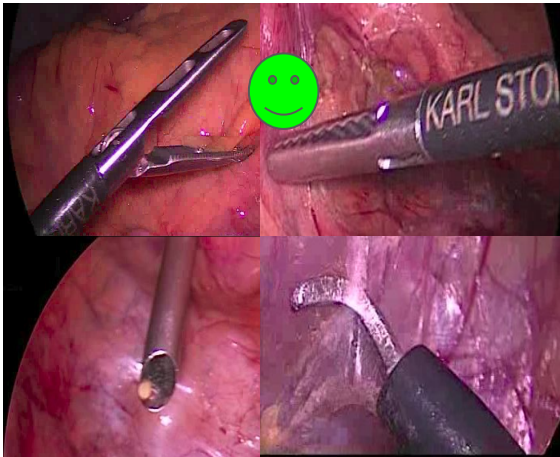

Examples of matter:  
surgical tools

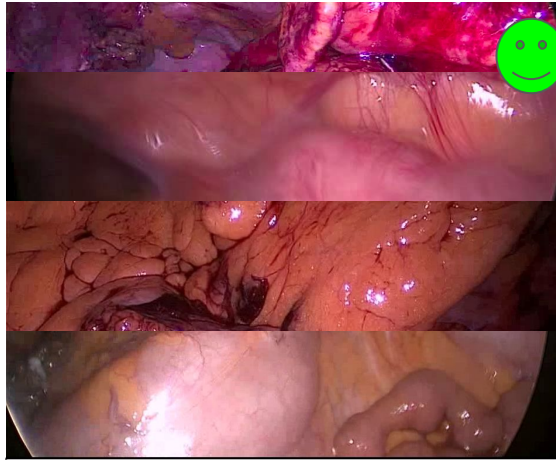

Examples of matter:  
Tissue

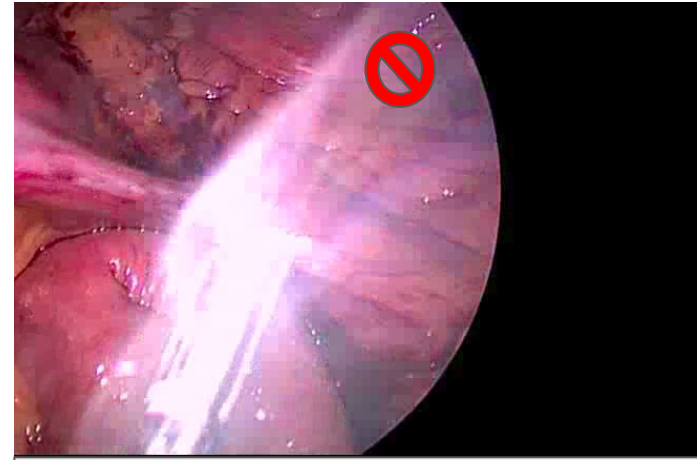

Counterexample:  
Smoke

# Goal - Detect and segment all relevant medical instruments

## Only segment medical instruments

- Each medical instrument is their own instance.
- If two parts of the same instrument are visible, they belong to the same instrument instance.
- Each instance has their own colour.

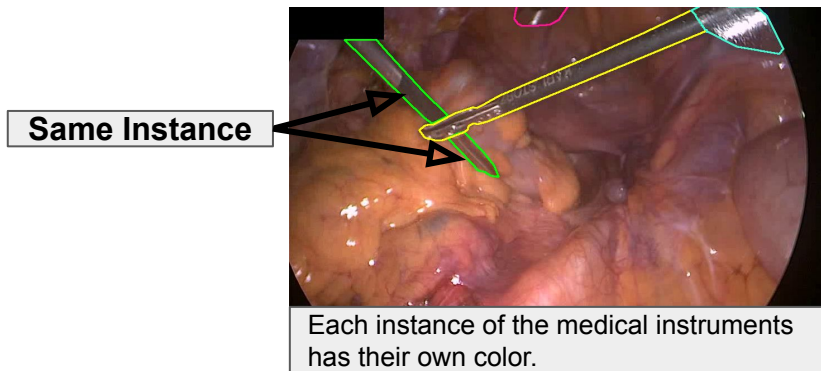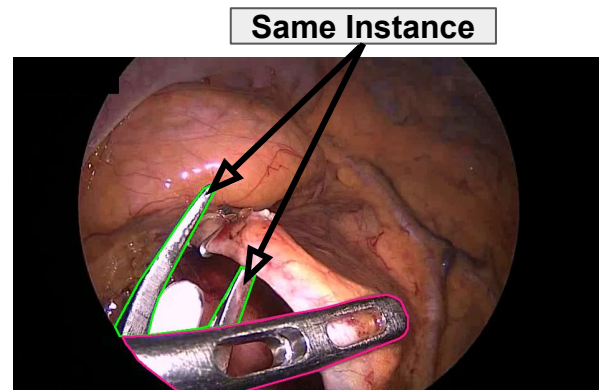

# Goal - Detect and segment all relevant medical instruments

## Only segment medical instruments

- The interior of a segmentation represents a medical instrument.
- Everything outside the medical instrument segmentations is regarded as other matter.
- Be as precise as possible. Every pixel counts in surgery.

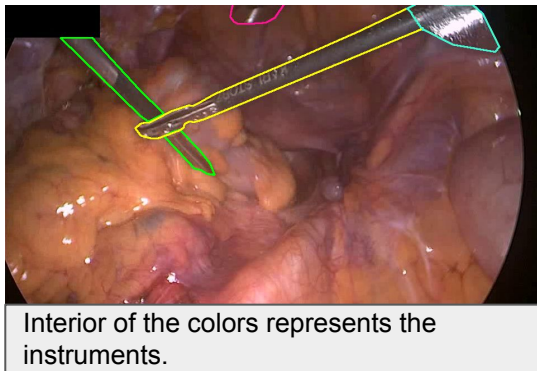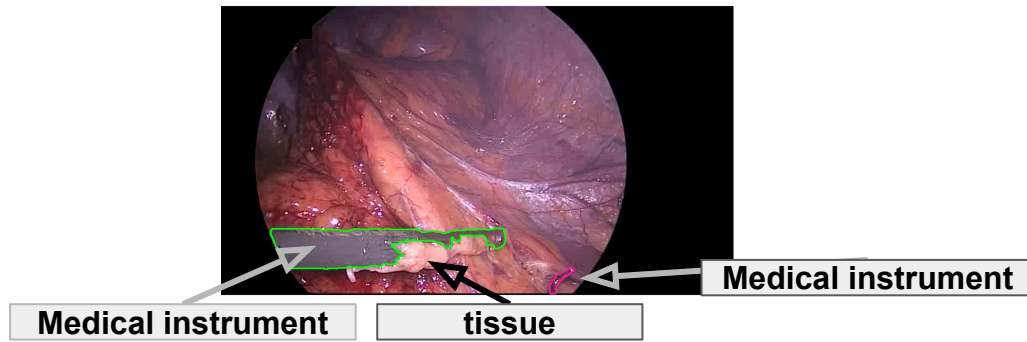

# Occlusion

Each pixel may correspond to exactly one instance.

- The solid/liquid matter that occurs first along the line of sight of the endoscope determines the label.

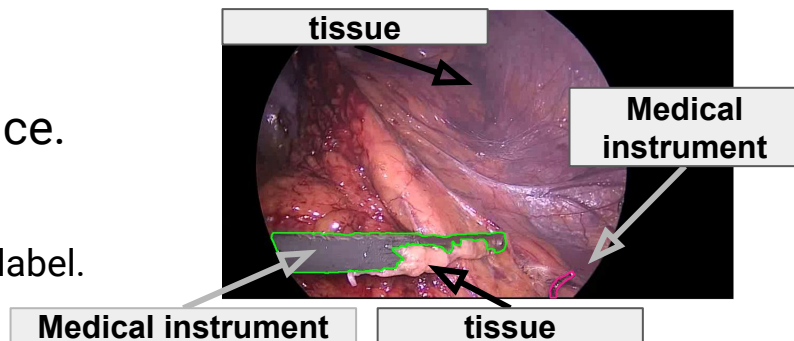

This may result in multiple segmentations for a single instrument that is occluded by another instrument, blood or tissue, for example.

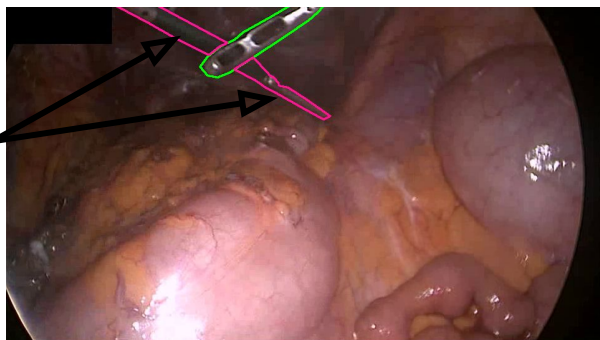

Pink is a medical instrument and occluded by green. -> Pink has two segmentations.

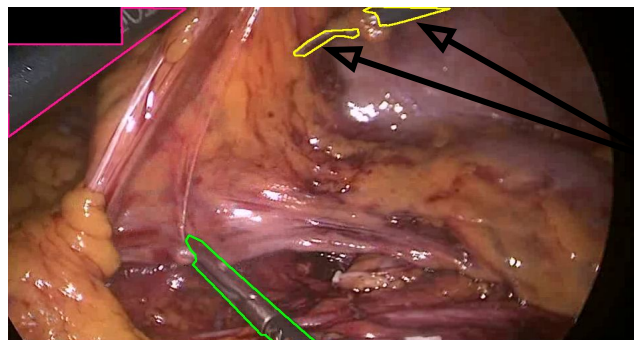

Pink is partly occluded by an image overlay. Yellow is occluded by tissue -> Two segmentations

# Medical instruments

## Definition “Medical instrument”:

- An elongated rigid object placed into the patient and manipulated from outside the patient.
- Examples: grasper, scalpel, (transparent) trocar, clip applicator, hooks, stapling device, suction

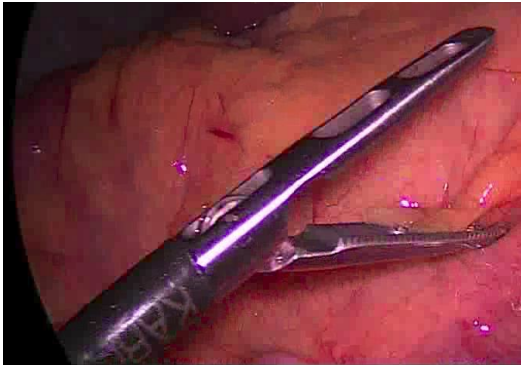

Example: Grasper

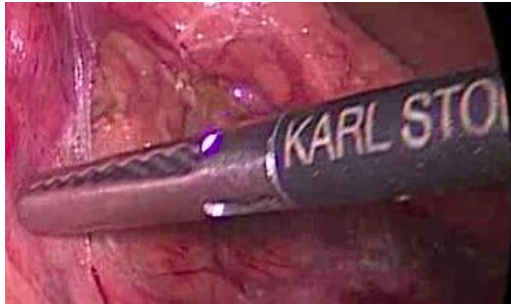

Example: Grasper

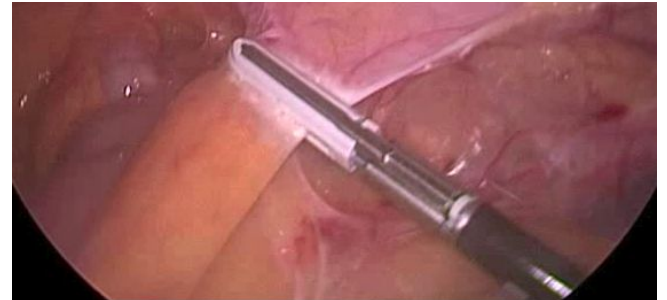

Example: Grasper



# Medical instruments

## Definition “Medical instrument”:

- An elongated rigid object placed into the patient and manipulated from outside the patient.
- Examples: grasper, scalpel, (transparent) trocar, clip applicator, hooks, stapling device, suction

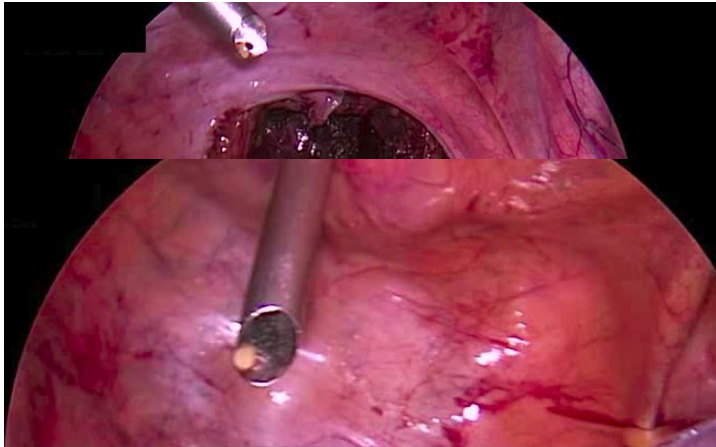

Example: Suction

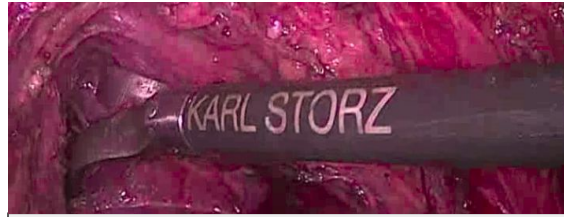

Example: Scalpel

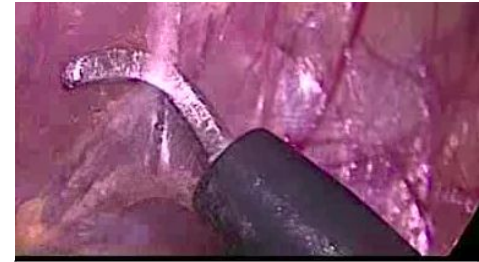

Example: Spreader

# Medical instruments

## Definition “Medical instrument”:

- An elongated rigid object placed into the patient and manipulated from outside the patient.
- Examples: grasper, scalpel, (transparent) trocar, clip applicator, hooks, stapling device, suction

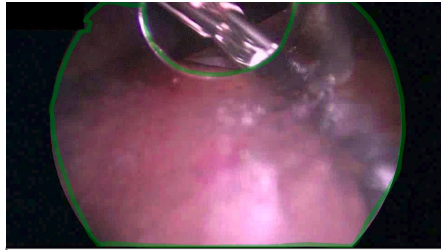

Example: Inside trocar (green). Another instrument is visible through the hole.

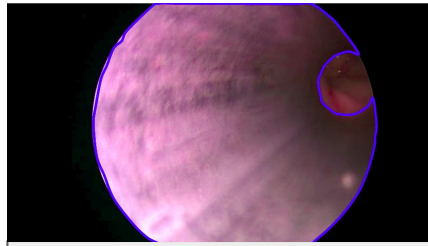

Example: Inside a Trocar

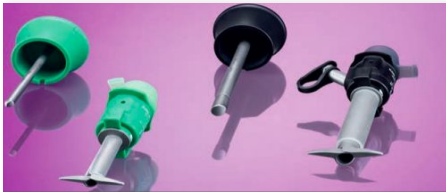

Example: Different trocars

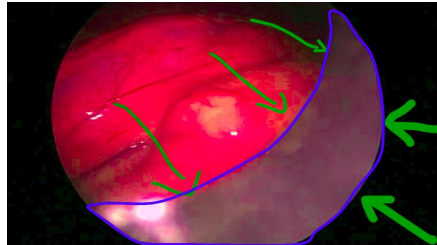

Example: Trocar

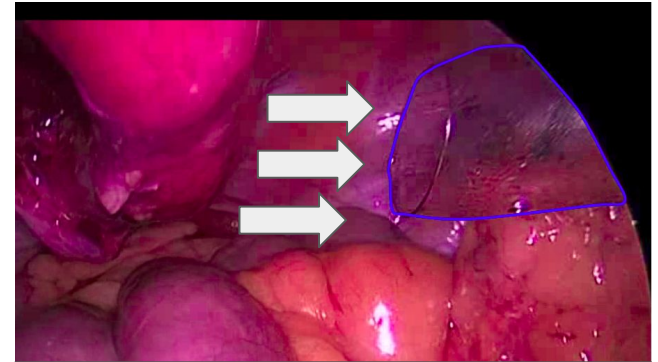

Example: transparent Trocar (hard to detect)



# Medical instruments

## Definition “Medical instrument”:

- Counterexamples: non-rigid tubes, bandage, compress, needle (not directly manipulated from outside but manipulated with an instrument), coagulation sponges, metal clips

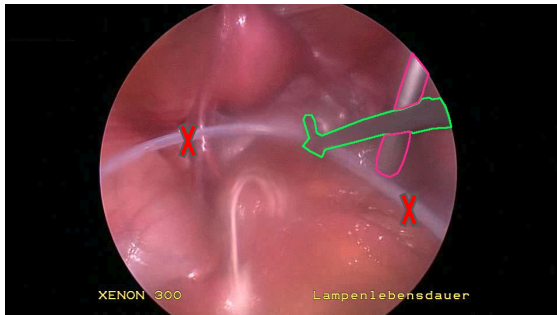

Green and pink are medical instruments.  
The red cross marks a drain-plastic  
-> no medical instrument

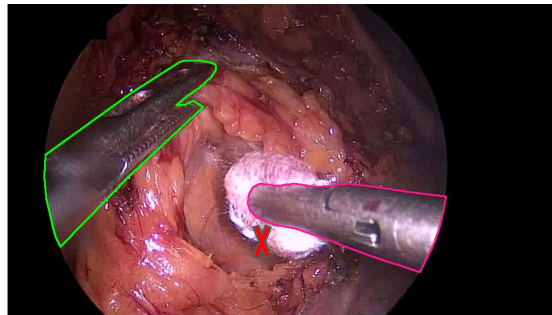

Green and pink are medical instruments.  
The red cross marks a bandage  
-> no medical instrument

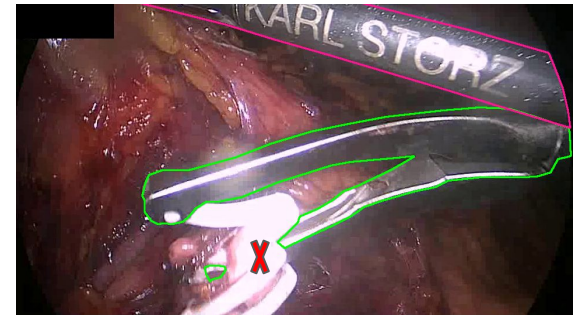

Green and pink are medical instruments.  
The red cross marks a clamp  
-> no medical instrument

# Medical instruments

## Definition “Medical instrument”:

- Counterexamples: non-rigid tubes, bandage, compress, needle (not directly manipulated from outside but manipulated with an instrument), coagulation sponges, metal clips

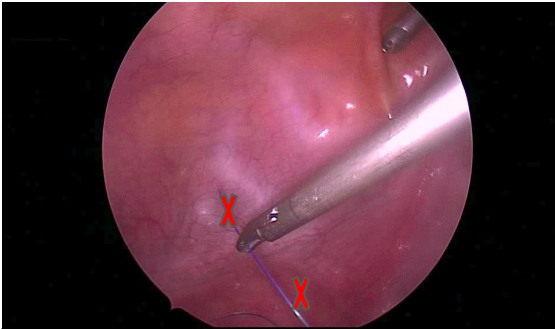

2 instruments are visible.  
The red cross marks a needle  
-> no medical instrument

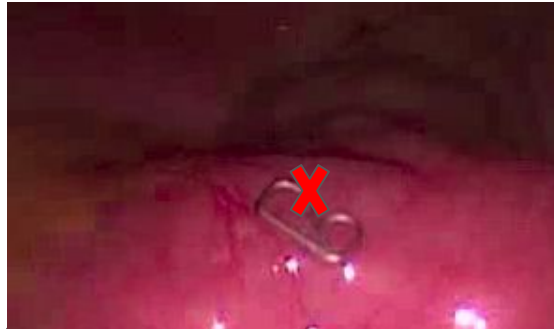

0 instruments are visible.  
The red cross marks a metal clip  
-> no medical instrument

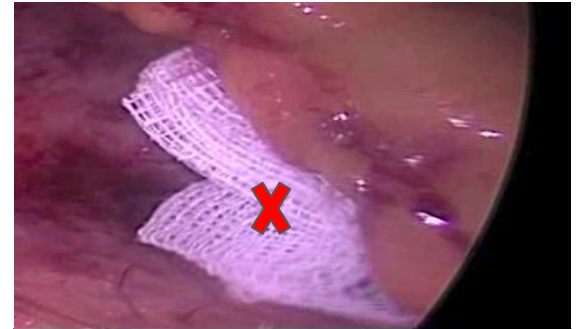

0 instruments are visible.  
The red cross marks a bandage  
-> no medical instrument

# Medical instruments - Holes

Several medical instruments feature holes.  
They are regarded as part of the instrument.

A hole is made up of pixels that do not show parts of the instrument but are either

type (a) completely surrounded by pixels of the same instrument or

type (b) are completely surrounded by pixels of one instrument and the margin of the instrument would close the hole outside the image.

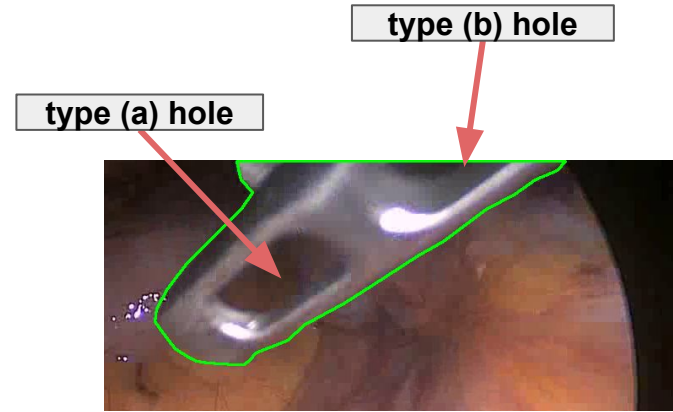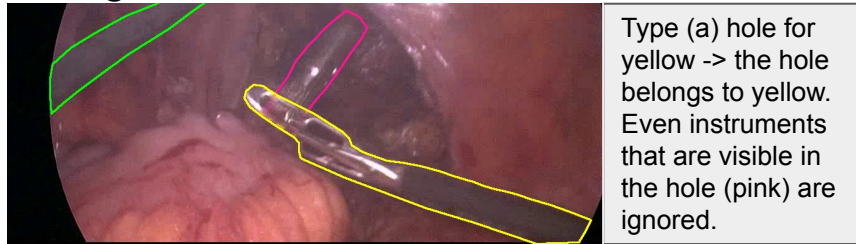

# Medical instruments - Holes exception

The sole exception are trocars when the camera is placed inside of them.

Trocars are transparent medical instruments.

- They are placed through the abdomen.
- To function as a portal for the other medical instruments.

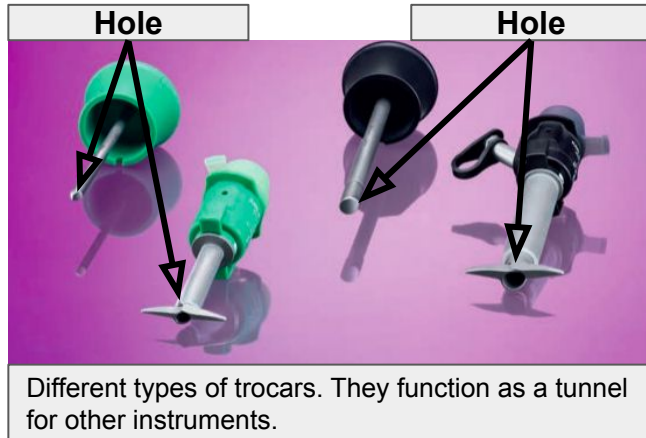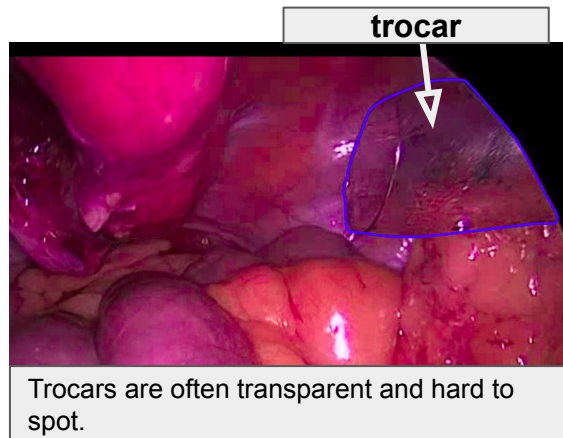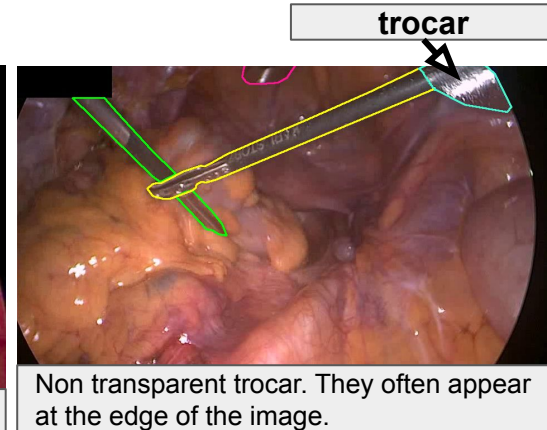

# Medical instruments - Holes exception

The sole exception are trocars when the camera is placed inside of them.

When the camera is inside a trocar, a trocar can take up a large part of the image

Trocars are exempt from the hole rule.

- Otherwise, the holes would contain a large part of the image.

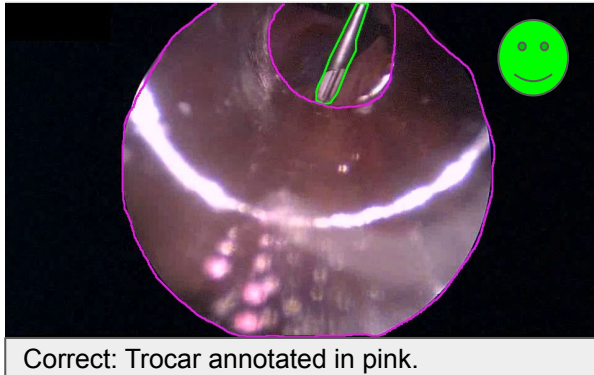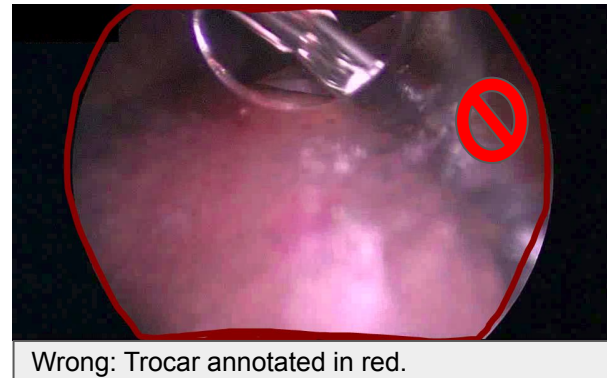

# Medical instruments - Transparency

Medical instruments may be transparent.

The occlusion rule holds in this case as well.

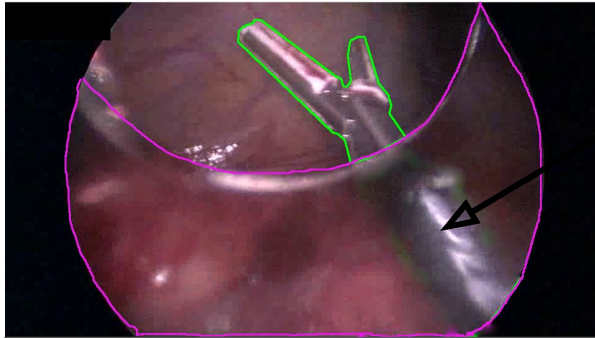

Hole exception for pink (tronicar). Pink is transparent. -> The hidden part of green belongs to the pink annotation (occlusion rule).

**Pixels only belong to one instrument.**

Here they belong to the transparent instrument, because the transparent instrument is the first object in line of sight (occlusion rule).

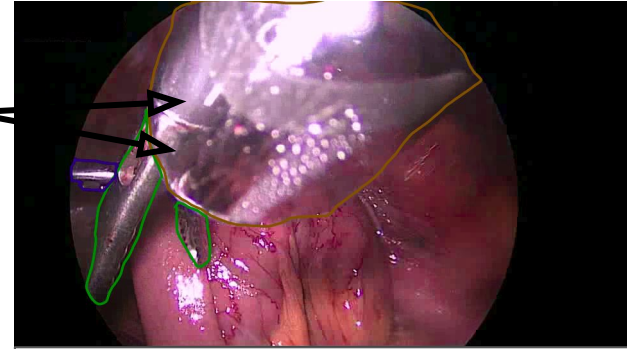

Green and blue are instruments. Brown is a transparent trocar. -> The trocar is the first part in the line of sight. Hidden part of the green instrument belongs to brown (occlusion rule).



# Text overlay

Text overlay is text that is visible in the image.  
The background of the text is the regular image.

Text overlay shall be ignored.

Examples:

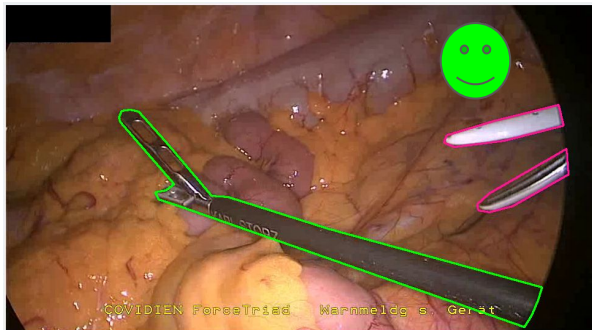

Correct: The text overlay is ignored.

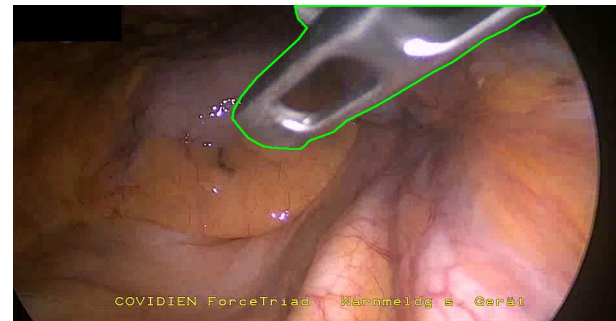

Text overlay (in yellow color)

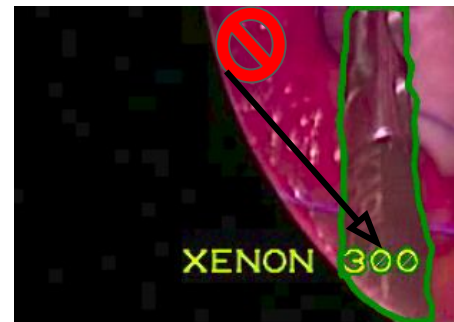

Wrong: The text overlay is treated with a cutout.

# Image overlay

Image overlay is often uniform coloured shapes that overlay on the image.

Text with a added uniform color background is considered as image overlay.

Image overlays are treated like “other matter”.

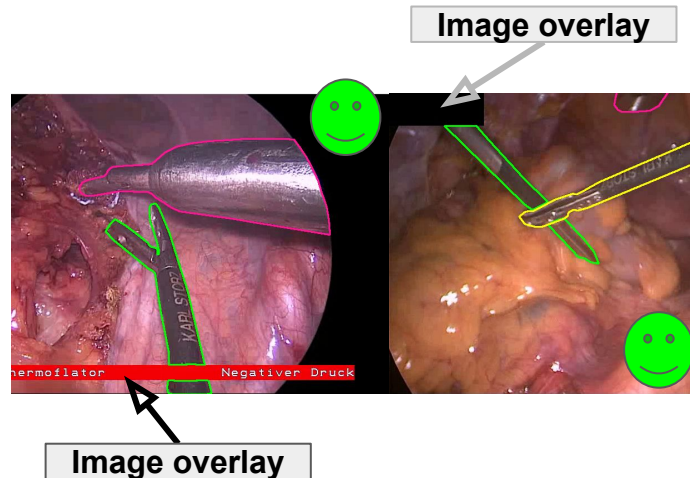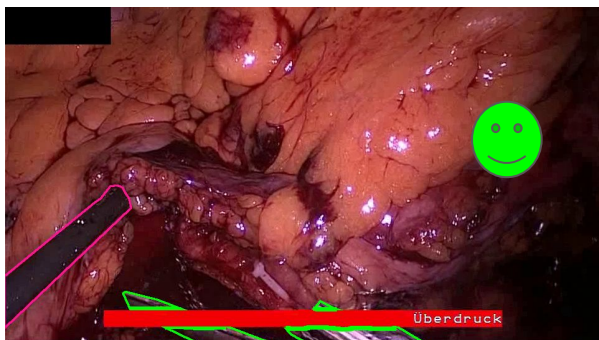

Correct: The image overlay is not part of the instrument.

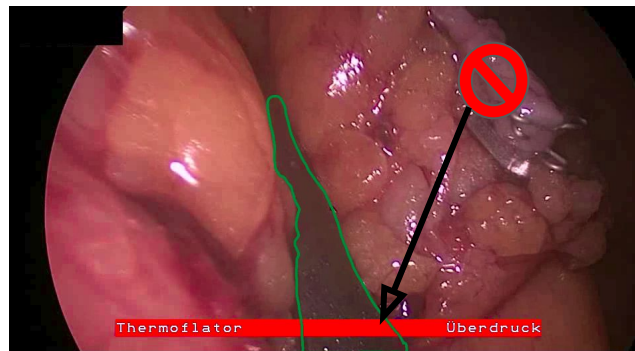

Wrong: The image overlay here part of the instrument.
